# Supplementary material for: On the Role of Attention in Prompt-tuning
Source: arXiv:2306.03435 source file (2023-06-06)
Supplement: Supplementary file 1 [file appendix.tex]

% \begin{fact}\label{fact:max subg}
%     Let $G_i,i\in[N]$ be \iid subgaussians with subgaussian constant $\sigma$. Then, $\max_{i\in[N]}g_i\leq\sqrt{\log}$
% \end{fact}

\section{Proofs}
